# Supplementary material for: On Generalized Degree Fairness in Graph Neural Networks
Source: arXiv:2302.03881 source file (2023-02-20)
Supplement: Supplementary file 1 [file sec-appendix.tex]

\setcounter{secnumdepth}{5}

% \section*{Appendix}

\subsection{Algorithm and Complexity} \label{app.alg}

In this section, we first provide an outline of the model training, then analyze its computational complexity.

\stitle{Algorithm.} We outline the model training for \model\ in Algorithm~\ref{alg.train}. 
In line 1, we initialize the parameters set $\Theta$. 
In line 2, the training set $\bV^{\text{tr}}$ is divided into $G_0$ and $G_1$ \wrt the predefined threshold $K$.
In lines 4--10, we calculate the layer-wise node representations for the training set $\bV^{\text{tr}}$. In particular, for a target node $v$ in layer $l$, the context embedding $\vec{c}^{l}_v$ is calculated in line 6, and the scaling and shifting vectors $\gamma^{l}_v$ and $\beta^{l}_v$ are calculated in line 7. Furthermore, the debiasing contexts for complementing (\ie, $\bD(v;\theta^l_0)$) and distilling (\ie, $\bD(v;\theta^l_1)$) are achieved in lines 8 and 9, respectively. Thereafter, we generate the node representation $\vec{h}^l_v$ based on the debiasing neighbor aggregation in line 10.
In lines 11--14, we compute the classification loss (line 11), fairness loss (line 12), constraints on debiasing contexts (line 13), and constraints on scaling and shifting vectors (line 14), respectively. Based on them, we formalize the overall objective $\bL$ in line 15. 
We optimize $\Theta$ by minimizing $\bL$ in line 16.

\begin{algorithm}[h]
\small
\caption{\textsc{Model Training for \model}}
\label{alg.train}
\begin{algorithmic}[1]
    \Require Graph $\bG=\{\bV, \bE, \vec{X}\}$, training set $\bV^{\text{tr}}$, threshold hyperpatameter $K$, and hyperparameters $\{\epsilon, \mu, \lambda\}$.
    \Ensure Model parameters $\Theta$. 
    \State $\Theta\leftarrow$ parameters initialization;
    \State Split training set $\bV^{\text{tr}}$ into $G_0$ and $G_1$ \wrt $K$; % \Comment{Eqs.~(5) and (6)}
    \While{not converged}
        \For{$l\in\{1, 2, \ldots, \ell\}$}
            \For{$v\in\bV^{\text{tr}}$}
                \State $\vec{c}^{l}_v\leftarrow\textsc{Pool}(\{\vec{h}^{l-1}_u:\forall u \in \bC_r(v)\})$;  
                %\State \Comment{Context embedding, Eq.~(7)}
                \State $\gamma^{l}_v \leftarrow \phi_\gamma(\delta^l(v);\theta^l_{\gamma}), \quad \beta^{l}_v \leftarrow \phi_\beta(\delta^l(v);\theta^l_{\beta})$;
                %\State \Comment{Scaling and shifting vectors, Eq.~(10)}
                \State $\bD(v;\theta^l_0)\leftarrow(\gamma^{l}_v+\vec{1})\odot f(\vec{c}^{l}_v;\theta^l_{c,0})+\beta^{l}_v$; 
                %\State \Comment{Debiasing context for complementing, Eq.~(9)}
                \State $\bD(v;\theta^l_1)\leftarrow(\gamma^{l}_v+\vec{1})\odot f(\vec{c}^{l}_v;\theta^l_{c,1})+\beta^{l}_v$; 
                %\State \Comment{Debiasing context for distilling, Eq.~(9)}
                % \State $\vec{h}^l_v \leftarrow \sigma\bigg(\textsc{Aggr}(\{\vec{h}^{l-1}_u: u\in\bN_v\};\omega^l) + \epsilon\cdot (I(v\in G_0)  \bD(v;\theta^l_{0}) + I(v\in G_1)  \bD(v;\theta^l_{1}))\bigg)$;            
                %\State \Comment{Debiasing neighborhood aggregation, Eq.~(11)}
                \State $\vec{h}^l_v \leftarrow$ debiasing neighbor aggregation by Eq.~\eqref{eq.aggr};
            \EndFor
        \EndFor
        \State $\bL_{1} \leftarrow -\textstyle\sum_{v\in \bV^{\text{tr}}}\sum_{y=1}^{|\bY|} [\vec{y}_{v}]_y \ln [\vec{h}^{\ell}_{v}]_y$; %\Comment{Classification loss, Eq.~(12)}
        \State $\bL_2 \leftarrow \textstyle\left\|{\textstyle\frac{1}{|G_0^\text{tr}|}}\sum_{v\in G_0^\text{tr}}\vec{h}^{\ell}_v-{\textstyle\frac{1}{|G_1^{\text{tr}}|}}\sum_{v\in G_1^{\text{tr}}}\vec{h}^{\ell}_v\right\|^2_2$; %\Comment{Fairness loss, Eq.~(13)}
        \State $\bL_3 \hspace{-1mm}\leftarrow \hspace{-1mm} \sum_{l=1}^{\ell}\sum_{v\in\bV_{\text{tr}}} \bigg(I(v\hspace{-1mm}\in\hspace{-1mm} G_0) \|\bD(v;\theta^l_{1})\|^2_2  + I(v\hspace{-1mm}\in\hspace{-1mm} G_1) \|\bD(v;\theta^l_{0})\|^2_2\bigg)$;   %\Comment{Constraints on debiasing contexts, Eq.~(14)}
        \State $\bL_4\leftarrow\sum_{l=1}^{\ell}\sum_{v\in\bV_{\text{tr}}}(\|\gamma^{l}_v\|^2_2 + \|\beta^{l}_v\|^2_2)$; 
        %\State \Comment{Constraints on scaling and shifting, Eq.~(15)}
        \State $\bL \leftarrow \bL_1 + \mu \bL_2 + \lambda\cdot(\bL_3 + \bL_4 + \Omega(\Theta))$; %\Comment{Overall objective, Eq.~(16)}
        \State Update $\Theta$ by minimizing $\bL$;
    \EndWhile
    \State \Return $\Theta$.
\end{algorithmic}
\end{algorithm}

\eat{
\begin{algorithm}[h]
\small
\caption{\textsc{Model Training for \model}}
\label{alg.train}
\begin{algorithmic}[1]
    \Require Graph $\bG=\{\bV, \bE, \vec{X}\}$, training set $\bV^{\text{tr}}$, threshold hyperpatameter $K$, and parameters $\{\epsilon, \mu, \lambda\}$.
    \Ensure Model parameters $\Theta$. 
    \State $\Theta\leftarrow$ parameters initialization;
    \State Split training set $\bV^{\text{tr}}$ into $G_0$ and $G_1$ \wrt $K$; \Comment{Eqs.~(5) and (6)}
    \While{not converged}
        \For{$l\in\{1, 2, \ldots, \ell\}$}
            \For{$v\in\bV^{\text{tr}}$}
                \State $\vec{c}^{l}_v\leftarrow\textsc{Pool}(\{\vec{h}^{l-1}_u:\forall u \in \bC_r(v)\})$;  
                \State \Comment{Context embedding, Eq.~(7)}
                \State $\gamma^{l}_v \leftarrow \phi_\gamma(\delta^l(v);\theta^l_{\gamma}), \quad \beta^{l}_v \leftarrow \phi_\beta(\delta^l(v);\theta^l_{\beta})$;
                \State \Comment{Scaling and shifting vectors, Eq.~(10)}
                \State $\bD(v;\theta^l_0)\leftarrow(\gamma^{l}_v+\vec{1})\odot f(\vec{c}^{l}_v;\theta^l_{c,0})+\beta^{l}_v$; 
                \State \Comment{Debiasing context for complementing, Eq.~(9)}
                \State $\bD(v;\theta^l_1)\leftarrow(\gamma^{l}_v+\vec{1})\odot f(\vec{c}^{l}_v;\theta^l_{c,1})+\beta^{l}_v$; 
                \State \Comment{Debiasing context for distilling, Eq.~(9)}
                \State $\vec{h}^l_v \leftarrow \sigma\bigg(\textsc{Aggr}(\{\vec{h}^{l-1}_u: u\in\bN_v\};\omega^l) 
                + \epsilon\cdot (I(v\in G_0)  \bD(v;\theta^l_{0}) + I(v\in G_1)  \bD(v;\theta^l_{1}))\bigg)$;            
                \State \Comment{Debiasing neighborhood aggregation, Eq.~(11)}
            \EndFor
        \EndFor
        \State $\bL_{1} \leftarrow -\textstyle\sum_{v\in \bV^{\text{tr}}}\sum_{y=1}^{|\bY|} [\vec{y}_{v}]_y \ln [\vec{h}^{\ell}_{v}]_y$; \Comment{Classification loss, Eq.~(12)}
        \State $\bL_2 \leftarrow \textstyle\left\|{\textstyle\frac{1}{|G_0^\text{tr}|}}\sum_{v\in G_0^\text{tr}}\vec{h}^{\ell}_v-{\textstyle\frac{1}{|G_1^{\text{tr}}|}}\sum_{v\in G_1^{\text{tr}}}\vec{h}^{\ell}_v\right\|^2_2$; \Comment{Fairness loss, Eq.~(13)}
        \State $\bL_3 \leftarrow  \textstyle\sum_{l=1}^{\ell}\sum_{v\in\bV_{\text{tr}}} \bigg(I(v\in G_0) \|\bD(v;\theta^l_{1})\|^2_2  + I(v\in G_1) \|\bD(v;\theta^l_{0})\|^2_2\bigg)$;   \Comment{Constraints on debiasing contexts, Eq.~(14)}
        \State $\bL_4\leftarrow\textstyle\sum_{l=1}^{\ell}\sum_{v\in\bV_{\text{tr}}}(\|\gamma^{l}_v\|^2_2 + \|\beta^{l}_v\|^2_2)$; 
        \State \Comment{Constraints on scaling and shifting, Eq.~(15)}
        \State $\bL \leftarrow \bL_1 + \mu \bL_2 + \lambda\cdot(\bL_3 + \bL_4 + \Omega(\Theta))$; \Comment{Overall objective, Eq.~(16)}
        \State Update $\Theta$ by minimizing $\bL$;
    \EndWhile
    \State \Return $\Theta$.
\end{algorithmic}
\end{algorithm}
}

\stitle{Complexity analysis.}
The debiasing neighborhood aggregation increases the computational cost. Taking \method{GCN} as base model, with everything else being the same, we compare the complexity of 1-layer neighborhood aggregation for one node in \method{GCN} and \modelS{GCN}.
Given a node $v$ with degree $d$, the complexity of \method{GCN} is $O(d)$ for neighborhood aggregation.
On the other hand, the debiasing neighborhood aggregation of \modelS{GCN} contains the following steps. 
(1) The calculation of context embedding $\vec{c}^l_v$: we use an operator of mean-pooling to aggregate the layer-$l$ contents in node $v$'s $r$-hop local context $\bC_r(v)$ with $r=1$, thus involving the complexity of $O(d)$.
(2) The calculation of scaling (\ie, $\gamma^l_v$) and shifting (\ie, $\beta^l_v$) vectors: we utilize degree encoding $\delta^l(v)$ to calculate the scaling and shifting vectors, with complexity $O(1)$ for both of them.
(3) The calculation of debiasing contexts, including both $\bD(v;\theta^l_0)$ and $\bD(v;\theta^l_1)$: they are computed based on the achieved context embedding and scaling and shifting vectors, thus resulting in complexity of $O(1)$.
(4) The calculation of debiasing neighborhood aggregation $\vec{h}^l_v$: with referring to the neighbors once again for neighborhood aggregation (\ie, operation $\textsc{Aggr}(\cdot)$), this step involves additional complexity of $O(d)$.
Overall, in the calculation of debiasing neighborhood aggregation, the complexity of \modelS{GCN} is $O(2d+2)$, which has the same computational scale with its base model \method{GCN}, only differing by a constant factor. 
Note that, this comparison is also appropriate for other GNNs and the corresponding \model s.

\subsection{Details of Datasets} \label{app.datasets}
% In this section, we introduce detailed experimental setup and implementation notes for the datasets, the base GNN models, the baselines, and our proposed \model s, respectively.

% \stitle{Datasets.}
We use two Wikipedia networks, namely \emph{Chameleon} and \emph{Squirrel} \cite{pei2019geom}, in which each node represents a Wikipedia  page, and each edge denotes a reference between two pages in either direction. Node features are derived from informative keywords in each page. Each node is associated with a number denoting the monthly traffic of the page.
% We split the nodes into five categories for \emph{Chameleon} and \emph{Squirrel} while two categories for \emph{Crocodile} \wrt their traffic number for node classification, and evaluate the structural fairness in accordance with the predictions. 
We split the nodes into five categories \wrt their traffic volume for node classification. %, and evaluate the structural fairness in accordance with the predictions. 
We also use a citation network \emph{EMNLP} \cite{ma2020copulagnn}, in which each node denotes a paper published in the EMNLP conference, and each edge denotes two papers that have been co-cited by at least two EMNLP papers.
% the co-cited relationship between two papers by at least two EMNLP papers. 
Node features are derived from the principal components of keywords in paper title/abstract and the year of publication. Each node is associated with a number denoting the citation from outside of EMNLP.
We split the nodes into two categories \wrt their outside EMNLP citation count for node classification.

% \stitle{Dataset split.}

\subsection{Details of Base GNN Models} \label{app.based-models}
We give detailed descriptions and settings for the base GNN models, including \method{GCN} \cite{kipf2016semi}, \method{GAT} \cite{velivckovic2017graph} and \method{GraphSAGE} \cite{hamilton2017inductive}.

\stitle{Descriptions.}
We describe the three base GNN models below.
\begin{itemize}[leftmargin=*]
  \item \method{GCN} \cite{kipf2016semi}: \method{GCN} relies on the convolutional operation of neighborhood aggregation to recursively incorporate information from the neighbors of a target node. In particular, it resorts to mean-pooling to aggregate information from neighbors to produce the node representations.
  \item \method{GAT} \cite{velivckovic2017graph}: \method{GAT} utilizes a self-attention based neighborhood aggregation in each layer, thus the neighbors can be assigned particular weights \wrt their content.
  \item \method{GraphSAGE} \cite{hamilton2017inductive}: \method{GraphSAGE} relies on a similar yet different way with \method{GCN} for neighborhood aggregation, by paying more attention to the information from the target node itself.
\end{itemize}

% , due to their optimal performance with these settings.
\stitle{Settings.}
Based on the proposed setup by the original papers, we further tune the parameters in order to achieve their optimal performance, including accuracy and fairness. 
For \method{GCN} \cite{kipf2016semi}, we set the dropout rate as 0.5, the coefficient of regularization as 0.0001, and the learning rate as 0.01. In particular, we set the hidden dimension of the first layer as 32 for Chameleon, 64 for Squirrel and 16 for EMNLP.
% , due to their optimal performance with these settings.
For \method{GAT} \cite{velivckovic2017graph}, we utilize a self-attention mechanism with two heads, and set the dropout rate as 0.5, the coefficient of regularization as 0.0001, the learning rate as 0.01, and the hidden dimension of the first layer as 16 for all the datasets.
For \method{GraphSAGE} \cite{hamilton2017inductive}, we use the mean-pooling as the aggregator, and set the dropout rate as 0.5, the coefficient of regularization as 0.0001, and the learning rate as 0.01. In particular, we further set the hidden dimension of the first layer as 32 for Chameleon and Squirrel while 16 for EMNLP.

\subsection{Details of Baselines} \label{app.baselines}

\stitle{Descriptions.}
We describe the baselines as follows.

\noindent (1) \emph{Degree-specific models.}
\begin{itemize}%[leftmargin=*]
  \item \method{DSGCN} \cite{tang2020investigating}: To address accuracy bias among nodes with different degrees, \method{DSGCN} proposes to employ different models for nodes with different degrees, thus they can improve the performance for all the nodes.
  \item \method{Residual2Vec} \cite{kojaku2021residual2vec}: \method{Residual2Vec} also addresses a similar problem with \method{DSGCN}, which tries to modulate the random walk \wrt the node degrees thus they can achieve balanced probability for node sampling for better accuracy on all the nodes.
\end{itemize} 
\noindent (1) \emph{Fairness-aware models.}
\begin{itemize}%[leftmargin=*]
  \item \method{FairWalk} \cite{rahman2019fairwalk}: \method{FairWalk} follows the same paradigm of \method{DeepWalk} \cite{perozzi2014deepwalk}, including paths sampling and node representation learning (\eg, by \method{word2vec} \cite{mikolov2013distributed}). In particular, they conduct a sensitive attribute guided walk for path sampling. In other words, when sampling from the neighbors, they first randomly select a sensitive attribute, then randomly select a node from the chosen attribute. 
  \item \method{CFC} \cite{bose2019compositional}: In virtue of the well-designed filters over the node representations, \method{CFC} can filter out the sensitive attributes from the node representations for debiasing. It further employs a discriminator to adversarially facilitate the identification of sensitive attributes.
  \item \method{FairGNN} \cite{dai2021say}: Similar to \method{CFC}, \method{FairGNN} also applies the adversarial training principle for the promotion of distinguishing  sensitive attributes from the node representations.
  \item \method{FairAdj} \cite{li2020dyadic}: For dyadic fairness which is a distinct problem from ours, \method{FairAdj} tries to learn a fair adjacency matrix with proper graph structural constraints to debias the sensitive attributes for fair link prediction, and maintain the prediction accuracy at the same time.
\end{itemize}

% \zeminC{这里要突出说明，对于FairGNN，我们调整他们的参数使得他们能够得到不错的fairness效果。}

\subsection{Hyper-Parameter Settings} \label{app.parameter-settings}

\stitle{General settings.}
For all the GNN-based models, we apply a two-layer architecture %, due to the empirical effectiveness 
\cite{kipf2016semi,hamilton2017inductive,velivckovic2017graph}.

\stitle{Settings of baselines.}
We tune the parameters for baselines based on the proposed settings from the original papers to achieve their optimal performance, including accuracy and fairness. 
For \method{DSGCN} \cite{tang2020investigating}, we implement the model ourselves based on the details illustrated in the paper, and set the hidden dimension of the first layer as 32, and the threshold $d_{max}$ to prevent long-tail issue of the degrees as 20.
For \method{Residual2Vec} \cite{kojaku2021residual2vec}, we choose the version of matrix factorization for model optimization, and set the hidden dimension of embeddings as 32, and length of context window as 10.
For \method{FairWalk} \cite{rahman2019fairwalk}, we sample 20 paths starting from each node with length 80, and set embedding dimension as 128 on Chameleon and Squirrel while 64 on EMNLP \wrt their performance.
For \method{CFC} \cite{bose2019compositional}, to achieve its optimal performance, we set the training steps of discriminator as 2 with 0.1 as its weight, and the hidden dimension of the first layer as 32 on all the three datasets.
For \method{FairGNN} \cite{dai2021say}, we set $\alpha=4$ (controlling the influence of the adversary to the GNN classifier) and $\beta$ (controlling the contribution of the covariance constraint to ensure fairness) as 1 for Chameleon, 0.01 for Squirrel, 10 for EMNLP, and the hidden dimension of the first layer as 32 on the three datasets.
For \method{FairAdj} \cite{li2020dyadic}, we replace the reconstruction loss to node classification loss for fair comparison, and set number of epochs for utility optimization $T_1$ as 100. In addition, on datasets Chameleon and Squirrel, we set the number of epochs for fairness optimization $T_2$ as 10, and $\eta$ as 0.2; on dataset EMNLP, we set $T_2$ as 5 and $\eta$ as 0.1.

\stitle{Settings of \model.}
We build \model s based on the three base GNN models including \method{GCN} \cite{kipf2016semi}, \method{GAT} \cite{velivckovic2017graph} and \method{GraphSAGE} \cite{hamilton2017inductive}, thus forming the extended versions including \modelS{GCN}, \modelS{GAT} and \modelS{SAGE}, respectively.
In particular, we employ a group of unified main parameters for all these three extensions, by setting $\lambda=0.0001$, learning rate as 0.01 and dropout rate as 0.5. We also uniformly tune the other parameters for them on each dataset: on Chameleon, we set the hidden dimension of the first layer as 32, $\epsilon=1$ and $\mu=0.001$; on Squirrel, the hidden dimension as 32, $\epsilon=0.01$ and $\mu=0.0001$; and on EMNLP, the hidden dimension as 16, $\epsilon=0.001$ and $\mu=0.01$. As an exception, we set the hidden dimension of the first layer as 16 for \modelS{GAT} on all the three datasets, and deploy the self-attention mechanism with three heads.

% \subsection{Settings and parameters.}
% 这里可以分成两段，第一段是讲述实验设置，第二段讲述参数设置

% To form the two contrasting groups of low- and high-degree nodes, we set the threshold hyperparameter $K$ to the mean of 1-hop degrees (as depicted in Eqs.~(5) and (6)). 
%For the contrastive training of the model, we utilize $K=\textsc{Mean}\{s_1(v):v\in\bV\}$ to split all the training nodes into two groups, namely, the rich-structured nodes (\ie, $\bV_{\text{r}}$) and scarce-structured nodes (\ie, $\bV_{\text{s}}$).

\subsection{Environment}
We implemented the proposed \model\ using Pytorch 1.6 in Python 3.6.5. All experiments were conducted on a Linux workstation with a 6-core 3.6GHz CPU, 128GB DDR4 memory and two RTX 2080Ti GPUs.
